# Supplementary material for: Improving transferability of 3D adversarial attacks with scale and shear transformations
Source: arXiv:2211.01093 source file (2022-11-02)
Supplement: Supplementary file 1 [file Appendix.tex]

\newpage
\section{Appendix}

 \begin{figure*}[!htbp]
\centering
\includegraphics[width=0.98\textwidth]{fig/result_exp.pdf}
\caption{Example of original samples and successful adversarial samples generated through our attack method in N-MNIST and MNIST dataset under untargeted attack. The penultimate layer threshold during attack is set to 2. In N-MNIST dataset, we squeeze the sample along time steps.}
\label{fig:res:adversarial_examples}
\end{figure*}
